# Supplementary material for: Learning 3D Shapes as Multi-Layered Height-maps using 2D Convolutional Networks
Source: arXiv:1807.08485 source file (2018-07-26)
Supplement: Supplementary file 1 [file 1512-supp.pdf]

# Supplementary material: Learning 3D Shapes as Multi-Layered Height-maps using 2D Convolutional Networks

Kripasindhu Sarkar<sup>1,2</sup>, Basavaraj Hampiholi<sup>2</sup>,  
Kiran Varanasi<sup>1</sup>, and Didier Stricker<sup>1,2</sup>

<sup>1</sup>DFKI Kaiserslautern    <sup>2</sup>Technische Universität Kaiserslautern  
{kripasindhu.sarkar,basavaraj.hampiholi,  
kiran.varanasi,didier.stricker}@dfki.de

## 1 Introduction

In this short document, we provide the supplementary information for the paper ‘Learning 3D Shapes as Multi-Layered Height-maps using 2D Convolutional Networks’ - referred as *Main Paper*.

## 2 Feature visualization

Figure 1 shows the visualization of the features of a few shapes.

## 3 Memory calculation

Table 1 and 2 provides the memory calculation used for *Table 3 (Right)*, *Main paper*.

## 4 ModelNet40 misclassified shapes

Table 4 shows some of the misclassified shapes for the ModelNet40 dataset.

## 5 Network for Multi-View DCGAN

Table 3 shows the network in details for the experiments with MV-DCGAN in *Section 5.5*, *Main paper*.

## References

1. Riegler, G., Ulusoy, A.O., Geiger, A.: Octnet: Learning deep 3d representations at high resolutions. In: Proceedings of the IEEE Conference on Computer Vision and Pattern Recognition. (2017)

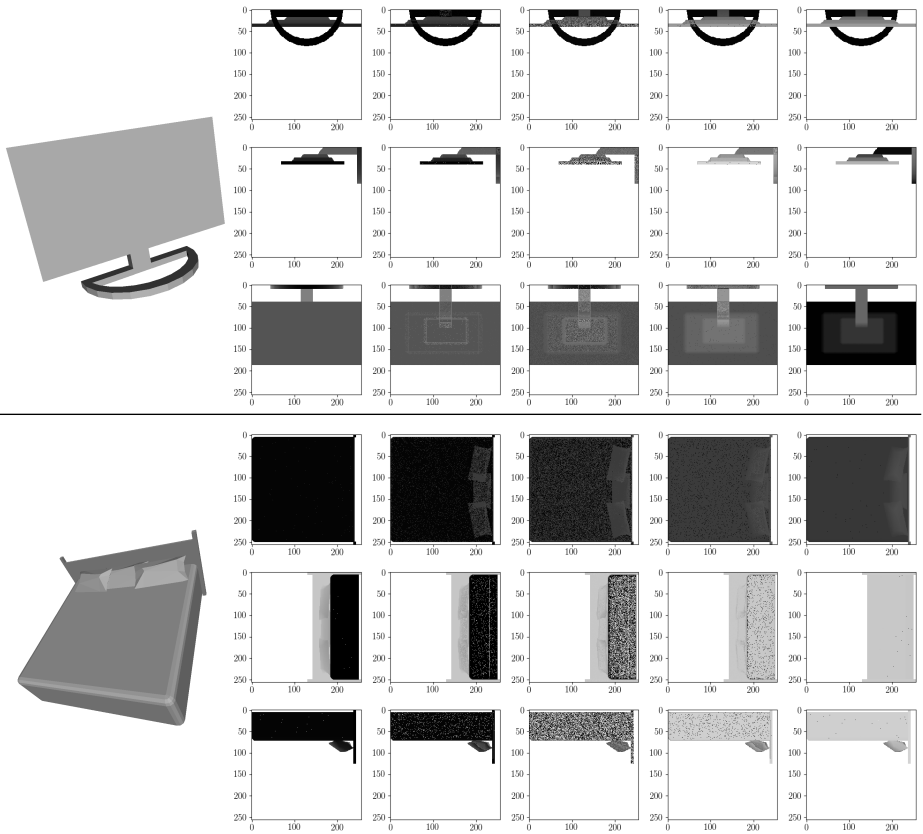

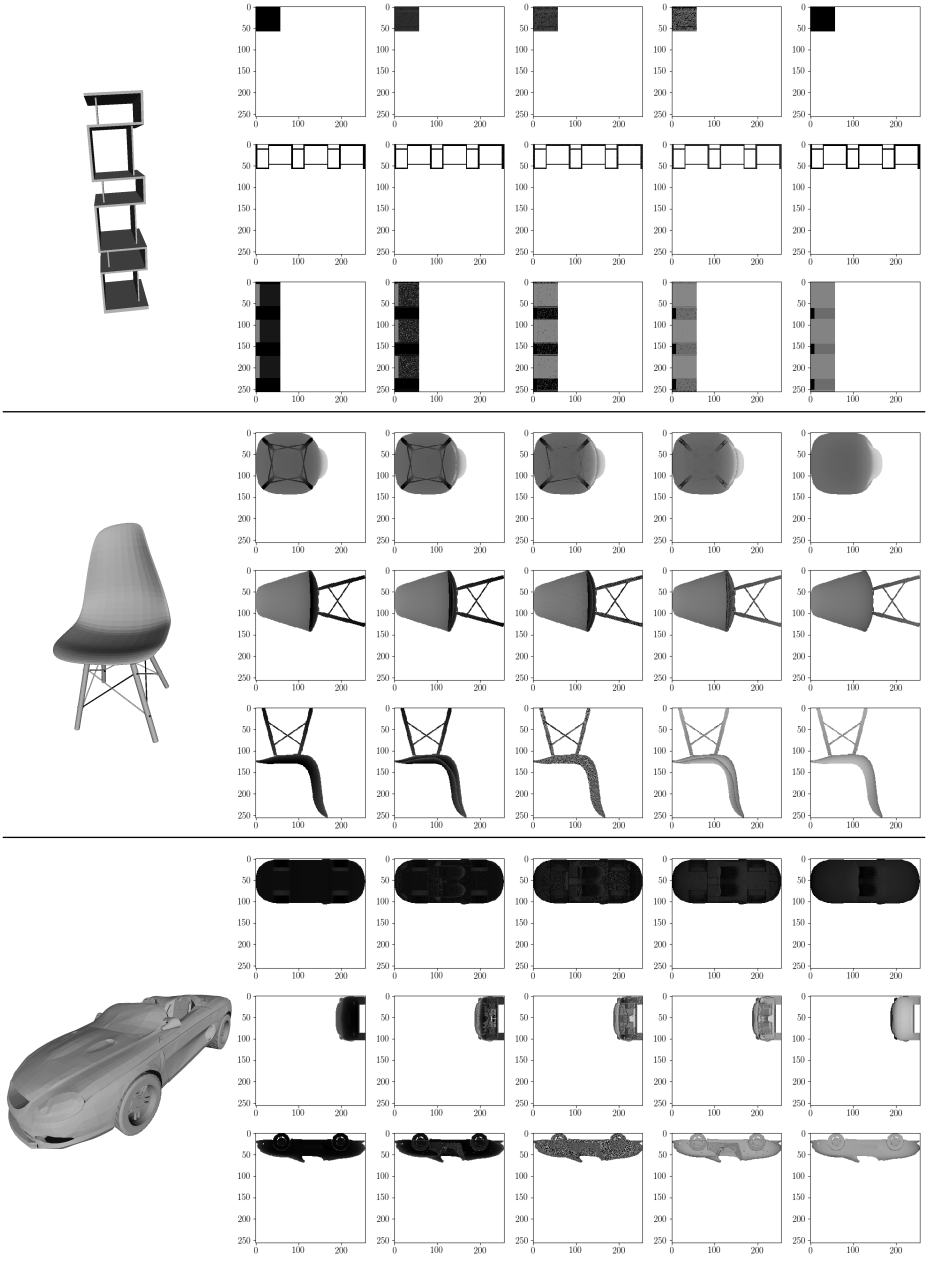

Fig. 1: Visualization of the multi-layered height-map descriptors of a few shapes. Each row represents a view direction (Z, X and Y in the order). Each column represent a layer (starting from 1 to 5). Note the distinctive features captured by the different layers - specially by the 1st and 5th layer. Eg, in the Z view of the car, tyres are captured by the 1st layer, hood and the roof by the 5th layer, while the seats and interiors like seats are captured by the intermediate layers.

| Network Architecture | Activation olume | Volume size | Memory                          |
|----------------------|------------------|-------------|---------------------------------|
| <i>input</i>         | 256x256x256x1    | 16777216    | 67108864                        |
| conv(1, 8)           | 256x256x256x8    | 134217728   | 536870912                       |
| conv(8, 14)          | 256x256x256x14   | 234881024   | 939524096                       |
| maxpool(2)           | 128x128x128x14   | 29360128    | 117440512                       |
| conv(14, 14)         | 128x128x128x14   | 29360128    | 117440512                       |
| conv(14, 20)         | 128x128x128x20   | 41943040    | 167772160                       |
| maxpool(2)           | 64x64x64x20      | 5242880     | 20971520                        |
| conv(20, 20)         | 64x64x64x20      | 5242880     | 20971520                        |
| conv(20, 26)         | 64x64x64x26      | 6815744     | 27262976                        |
| maxpool(2)           | 32x32x32x26      | 851968      | 3407872                         |
| conv(26, 26)         | 32x32x32x26      | 851968      | 3407872                         |
| conv(26, 32)         | 32x32x32x32      | 1048576     | 4194304                         |
| maxpool(2)           | 16x16x16x32      | 131072      | 524288                          |
| conv(32, 32)         | 16x16x16x32      | 131072      | 524288                          |
| conv(32, 32)         | 16x16x16x32      | 131072      | 524288                          |
| maxpool(2)           | 8x8x8x32         | 16384       | 65536                           |
| <b>Total</b>         |                  | 507002880   | 2028011520<br>$\approx 1.89$ GB |

Table 1: Memory computation for DenseNet256[1] for one sample. For a batch size of 32 we get  $32 \times 1.8 \approx 60$ GB of memory (*Table 3, Main Paper*). This value is also verified against the values in the plot provided in Figure 7(a) [1]

| Network Architecture  | Activation Volume | Volume size | Memory                   |
|-----------------------|-------------------|-------------|--------------------------|
| input                 | 256x256x5         | 327680      | 1310725                  |
| conv(5,64)            | 256x256x64        | 4194304     | 16777221                 |
| conv(64,64)           | 256x256x64        | 4194304     | 16777221                 |
| maxpool(2)            | 128x128x64        | 1048576     | 4194309                  |
| conv(64,128)          | 128x128x128       | 2097152     | 8388613                  |
| conv(128,128)         | 128x128x128       | 2097152     | 8388613                  |
| maxpool(2)            | 64x64x128         | 524288      | 2097157                  |
| conv(128,256)         | 64x64x256         | 1048576     | 4194309                  |
| conv(256,256)         | 64x64x256         | 1048576     | 4194309                  |
| conv(256,256)         | 64x64x256         | 1048576     | 4194309                  |
| maxpool(2)            | 32x32x256         | 262144      | 1048581                  |
| conv(256,512)         | 32x32x512         | 524288      | 2097157                  |
| conv(512,512)         | 32x32x512         | 524288      | 2097157                  |
| conv(512,512)         | 32x32x512         | 524288      | 2097157                  |
| maxpool(2)            | 16x16x512         | 131072      | 524293                   |
| conv(512,512)         | 16x16x512         | 131072      | 524293                   |
| conv(512,512)         | 16x16x512         | 131072      | 524293                   |
| conv(512,512)         | 16x16x512         | 131072      | 524293                   |
| maxpool(2)            | 8x8x512           | 32768       | 131077                   |
| <i>Total (branch)</i> |                   |             | 80084992 $\approx$ 80 MB |
| FC1                   | 1x1x4096          | 4096        | 16389                    |
| FC2                   | 1x1x4096          | 4096        | 16389                    |
| FC3                   | 1x1x40            | 40          | 165                      |
| <b>Total</b>          |                   |             | $\approx$ 112 MB.        |

Table 2: Memory computation for Our single view net using VGG for one sample. For a batch size of 32 we get  $32 \times 112 \approx 3.5$ GB of memory. But our experiments which was run using a PyTorch implementation for a batchsize of 32 occupies 8 GB of data in GeForce GTX 1080 Ti. We used this relaxed value of 8GB in *Table 3 (Right), Main Paper* for a more fare comparison against OctNet[1]. For OctNet we used the memory consumed in a similar settings using their representation and varified its value in the plot provided in the Figure 7(a) of [1].

|                         |                         |
|-------------------------|-------------------------|
| <i>input</i> - 100x1    |                         |
| convT(4x4, 512)         |                         |
| ReLU                    |                         |
| convT(4x4, 256, (2,2))  | <i>input</i> - 64x64x5  |
| ReLU                    | conv(4x4, 64, (2,2))    |
| convT(4x4, 128, (2,2))  | LReLU(0.2)              |
| ReLU                    | conv(4x4, 128, (2,2))   |
| convT(4x4, 64, (2,2))   | LReLU(0.2)              |
| ReLU                    | conv(4x4, 256, (2,2))   |
| convT(4x4, 5, (2,2))    | LReLU(0.2)              |
| Tanh                    | conv(4x4, 512, (2,2))   |
| <i>output</i> - 64x64x5 | <i>output</i> - 8x8x512 |

Table 3: (Left) The generative branch of the Multiview DCGAN which produces MLH vector of size 64x64x5. (Right) The discriminator part of the MV DCGAN which takes the generated 64x64x5 input and produces an activation volume of 8\*8\*512. In the multiview design we have 3 independent generator branches and 3 independent discriminator branches. The 3 output volume of the discriminator of the discriminator is concatenated by a non-commutative operation followed by FC(1024) and FC(1). More details are in *Figure 4, Main paper*. The number in the bracket (x,x) denotes the stride values for the strided convolution and and transposed convolution blocks. Batch-normalization is used between every layers except for the first and the last layers.

| GT label    | Predicted label | Misclassified shape                                                                 | Sample from predicted label                                                         |
|-------------|-----------------|-------------------------------------------------------------------------------------|-------------------------------------------------------------------------------------|
| plant       | flower pot      | 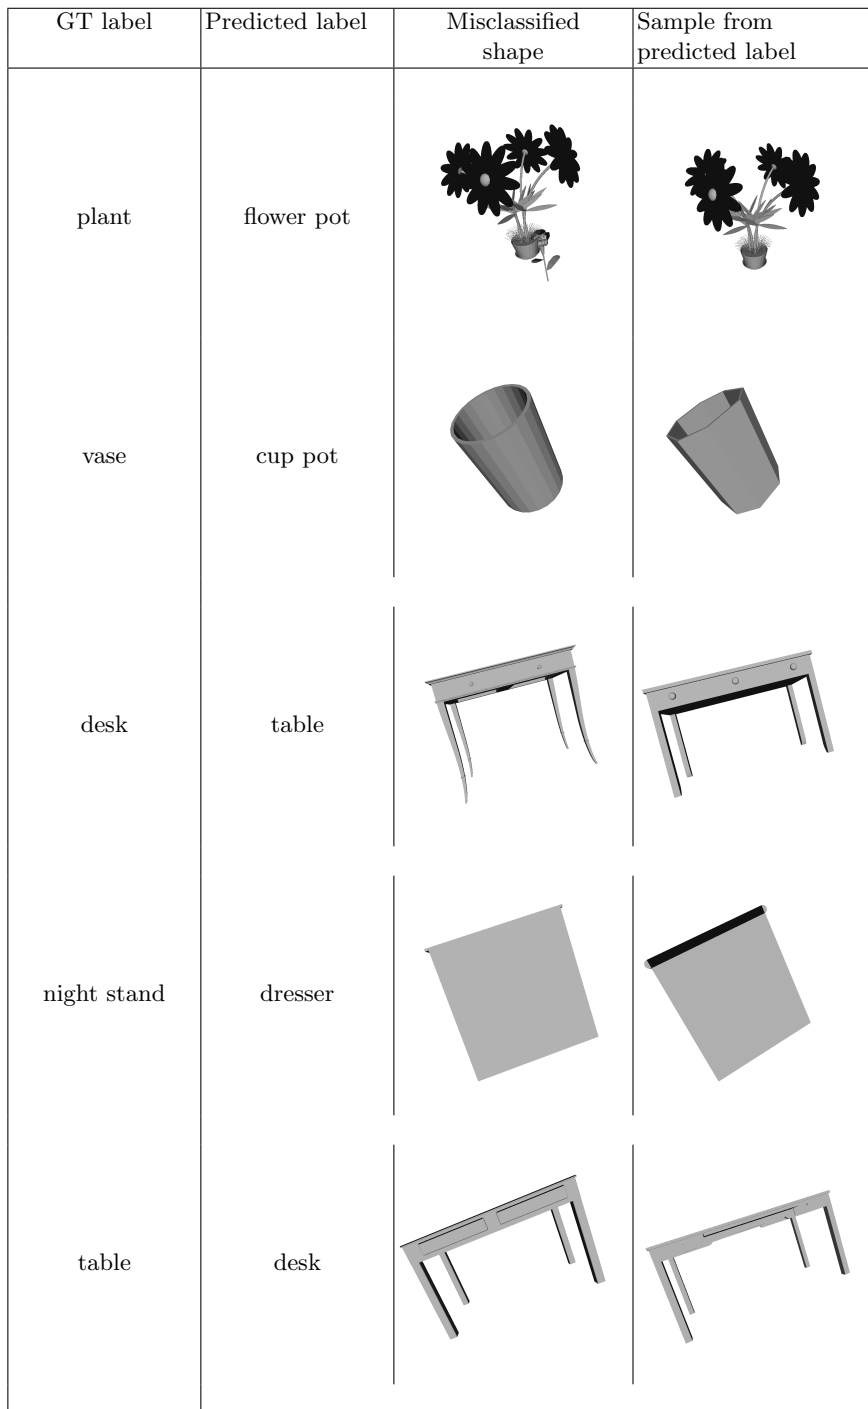   | 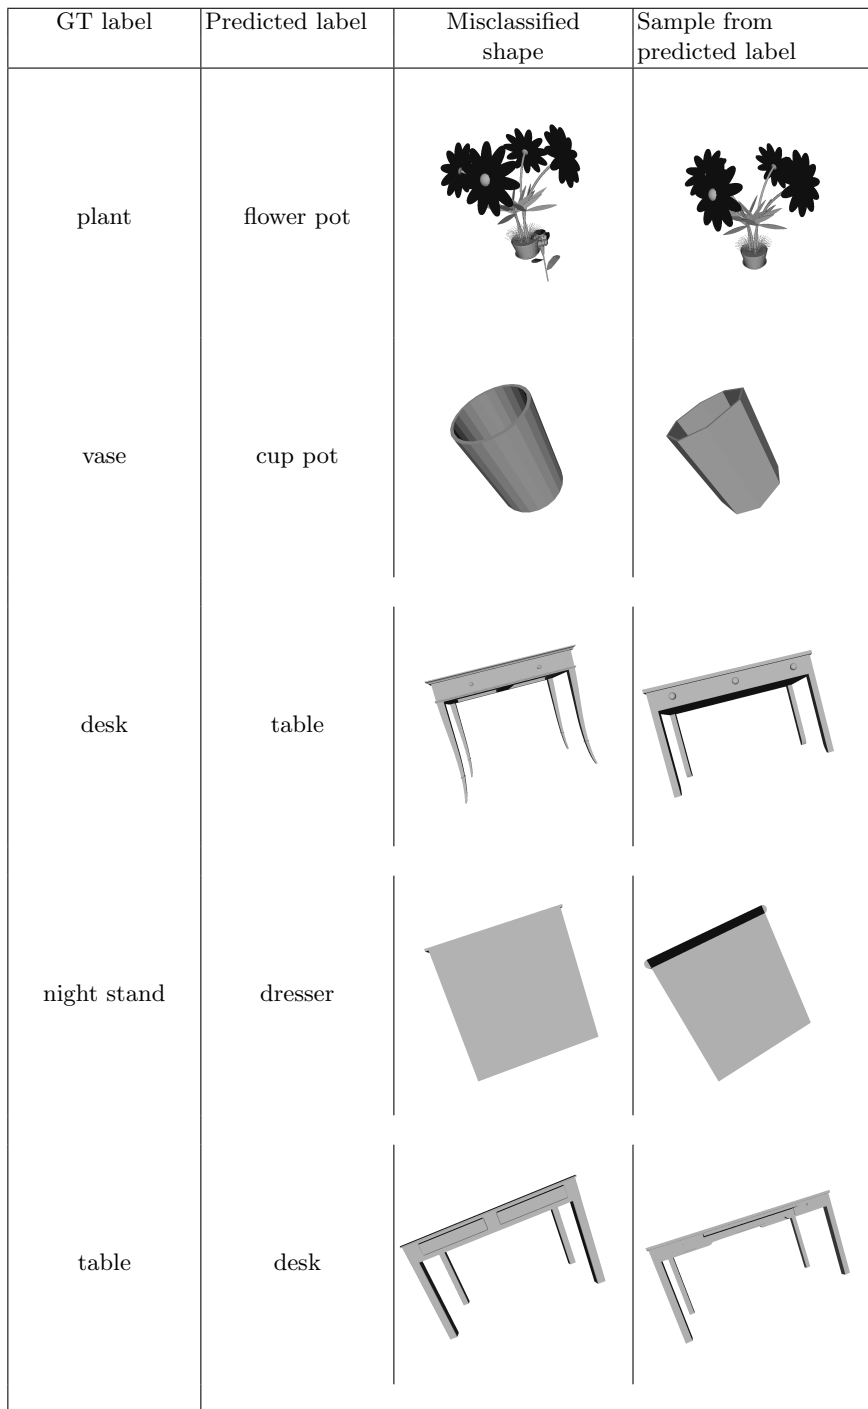   |
| vase        | cup pot         | 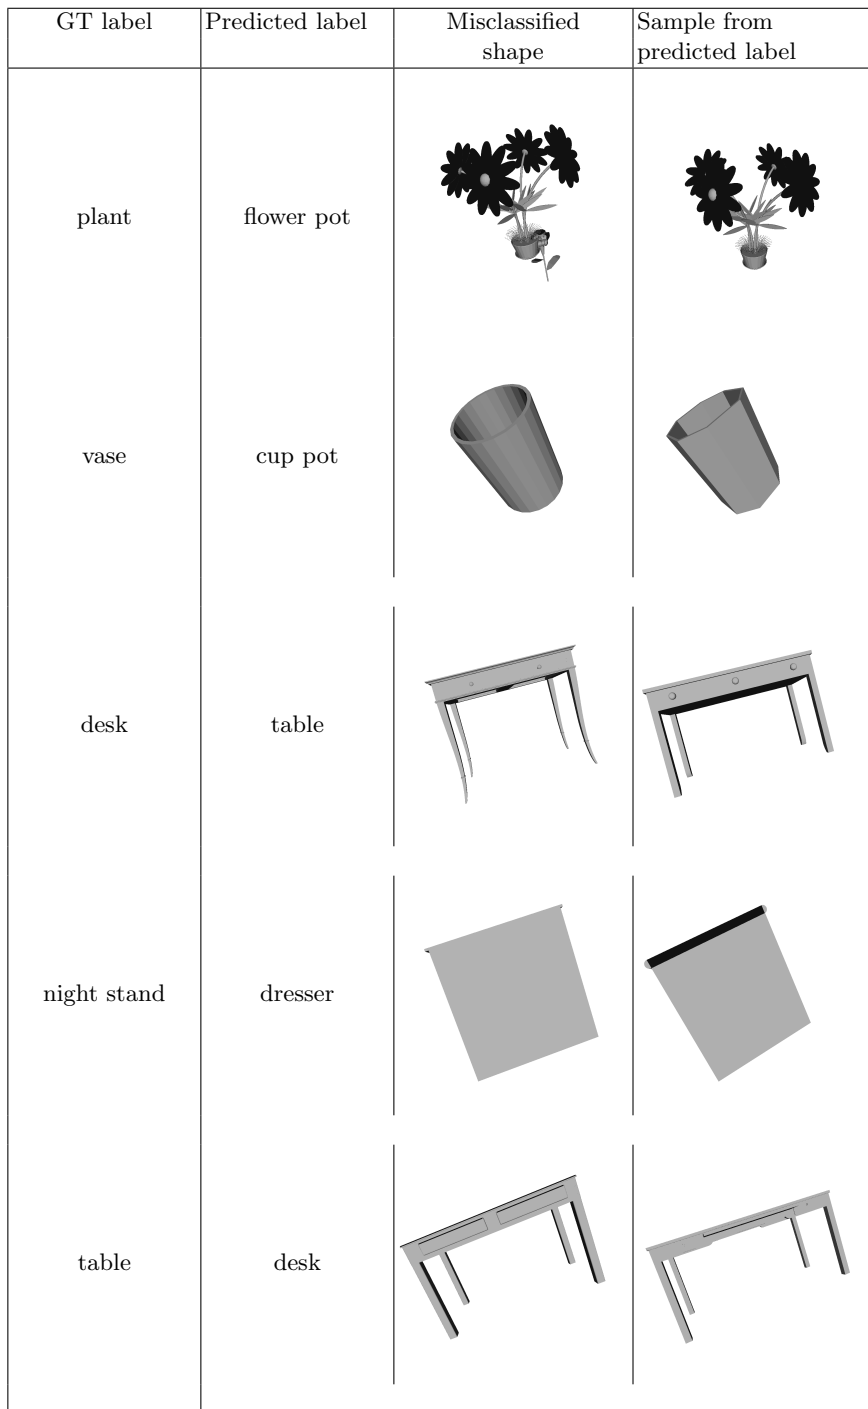   | 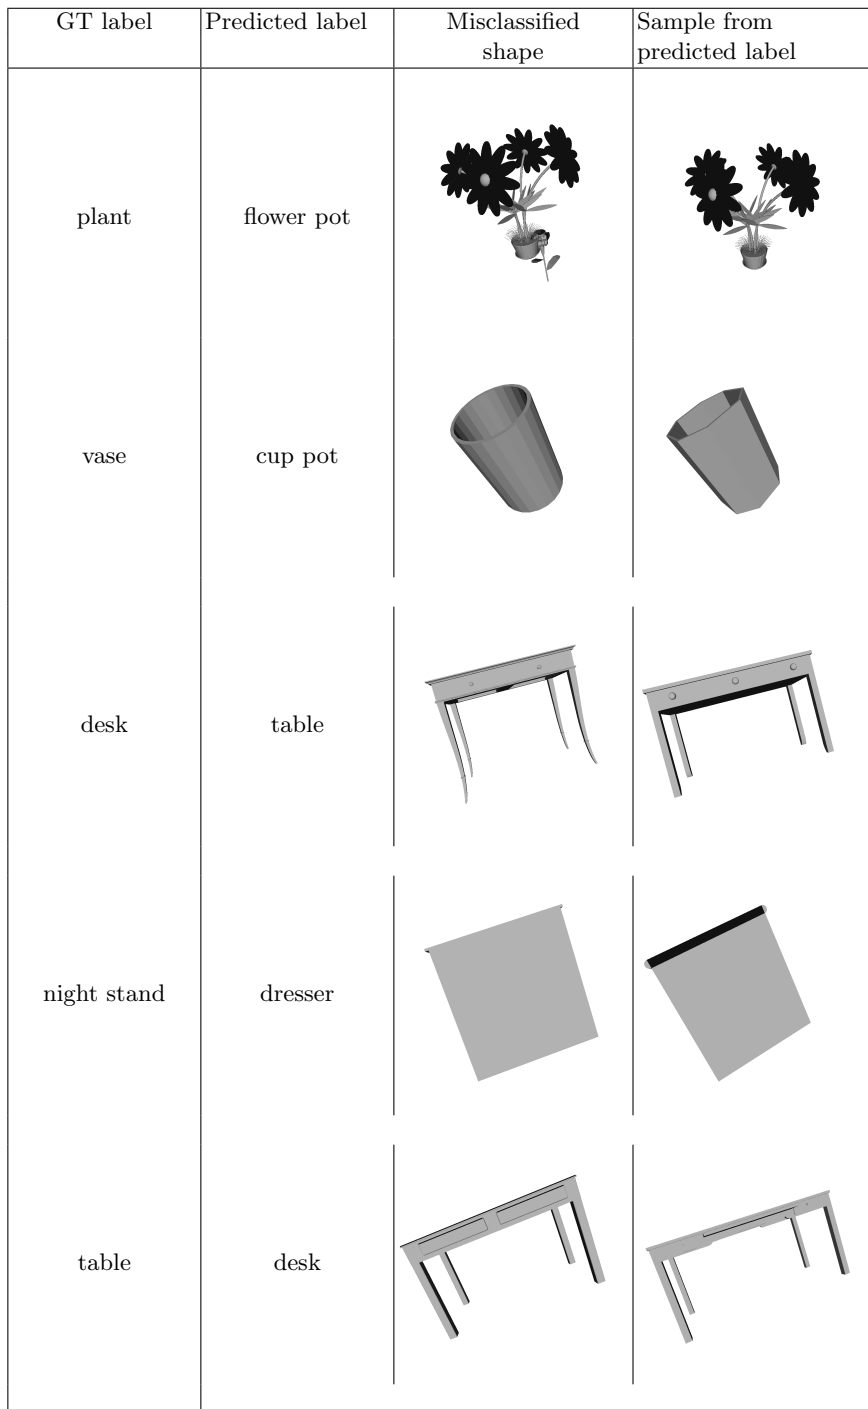   |
| desk        | table           | 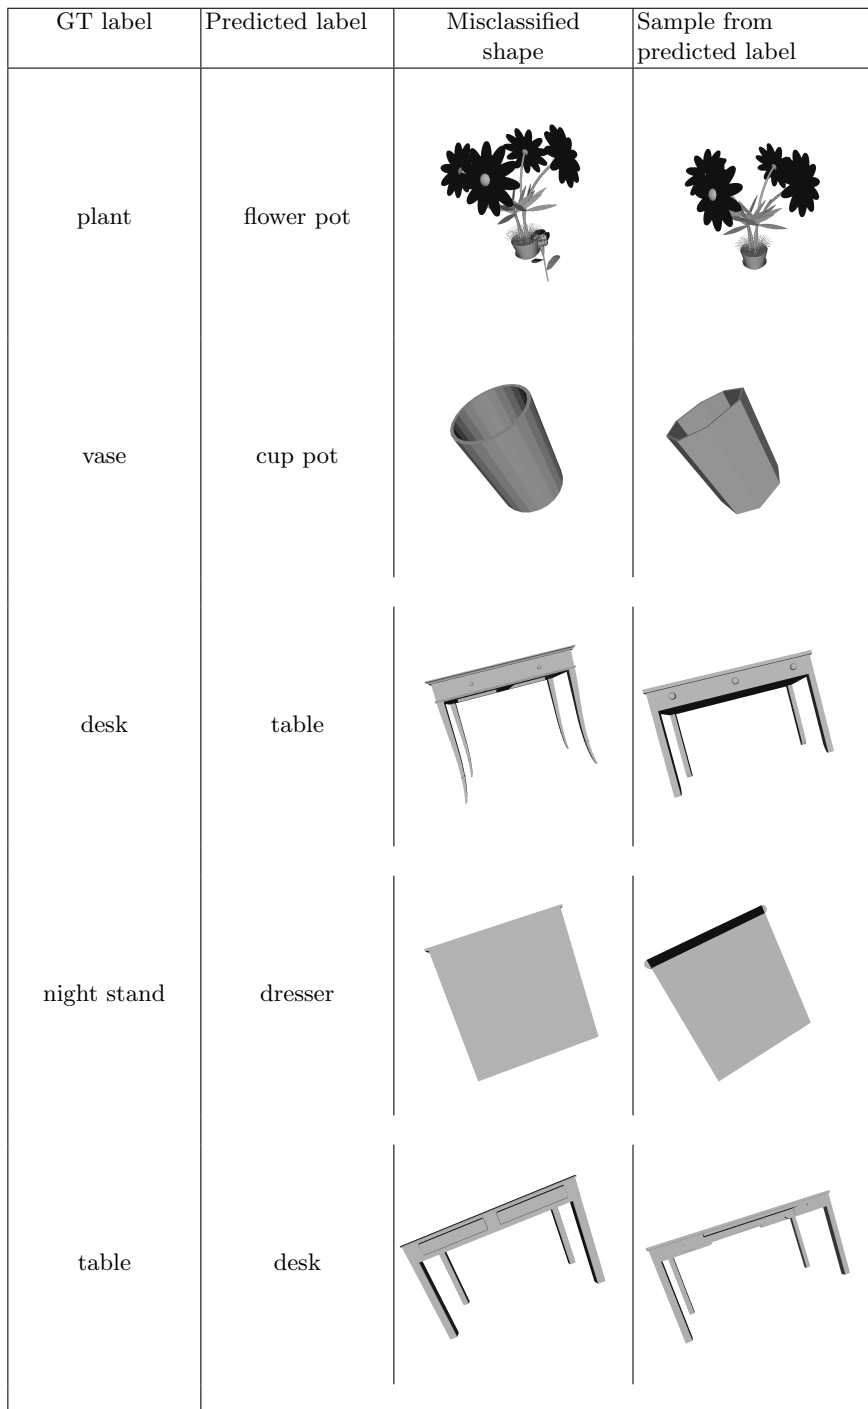   | 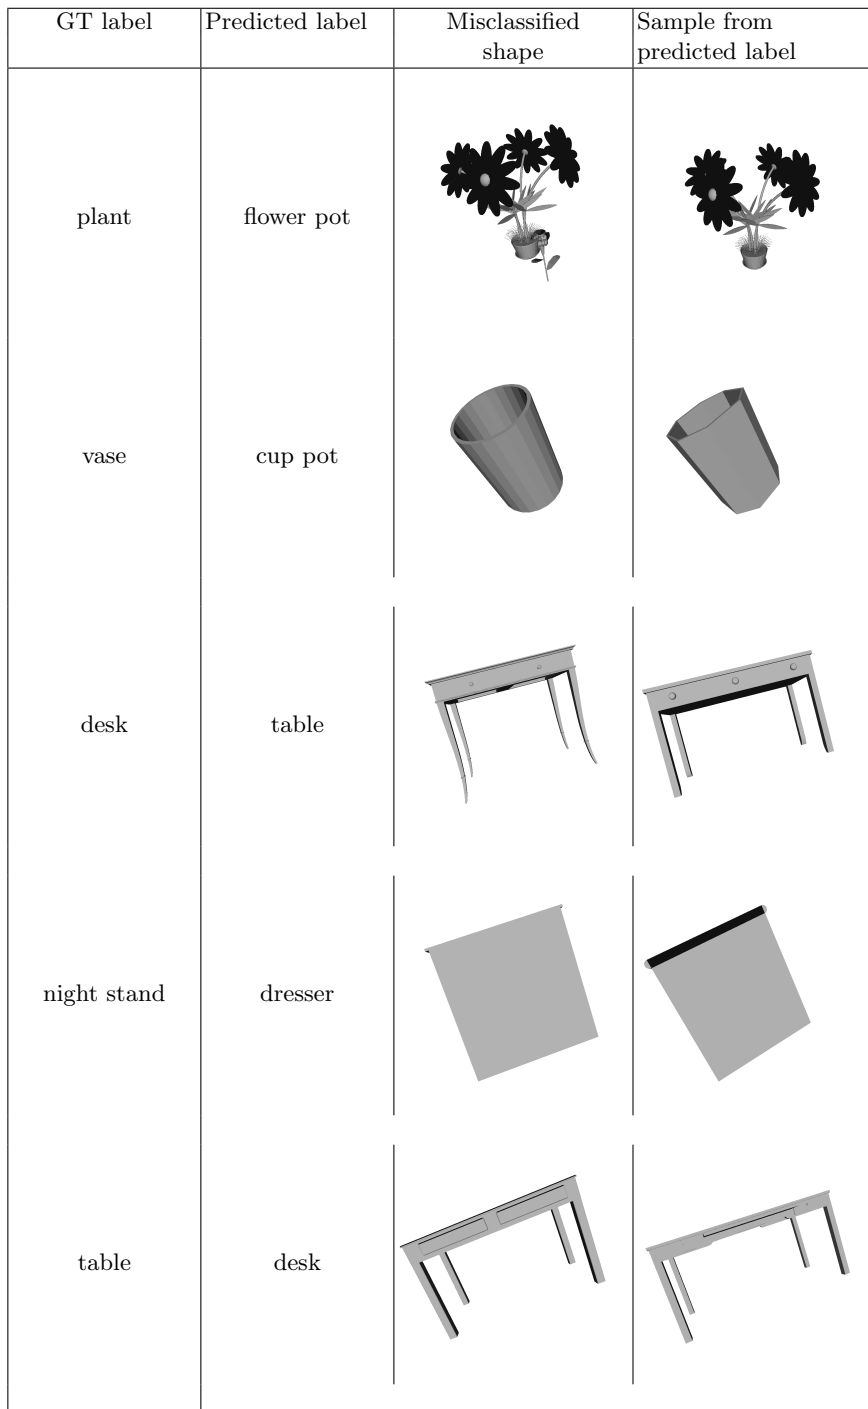   |
| night stand | dresser         | 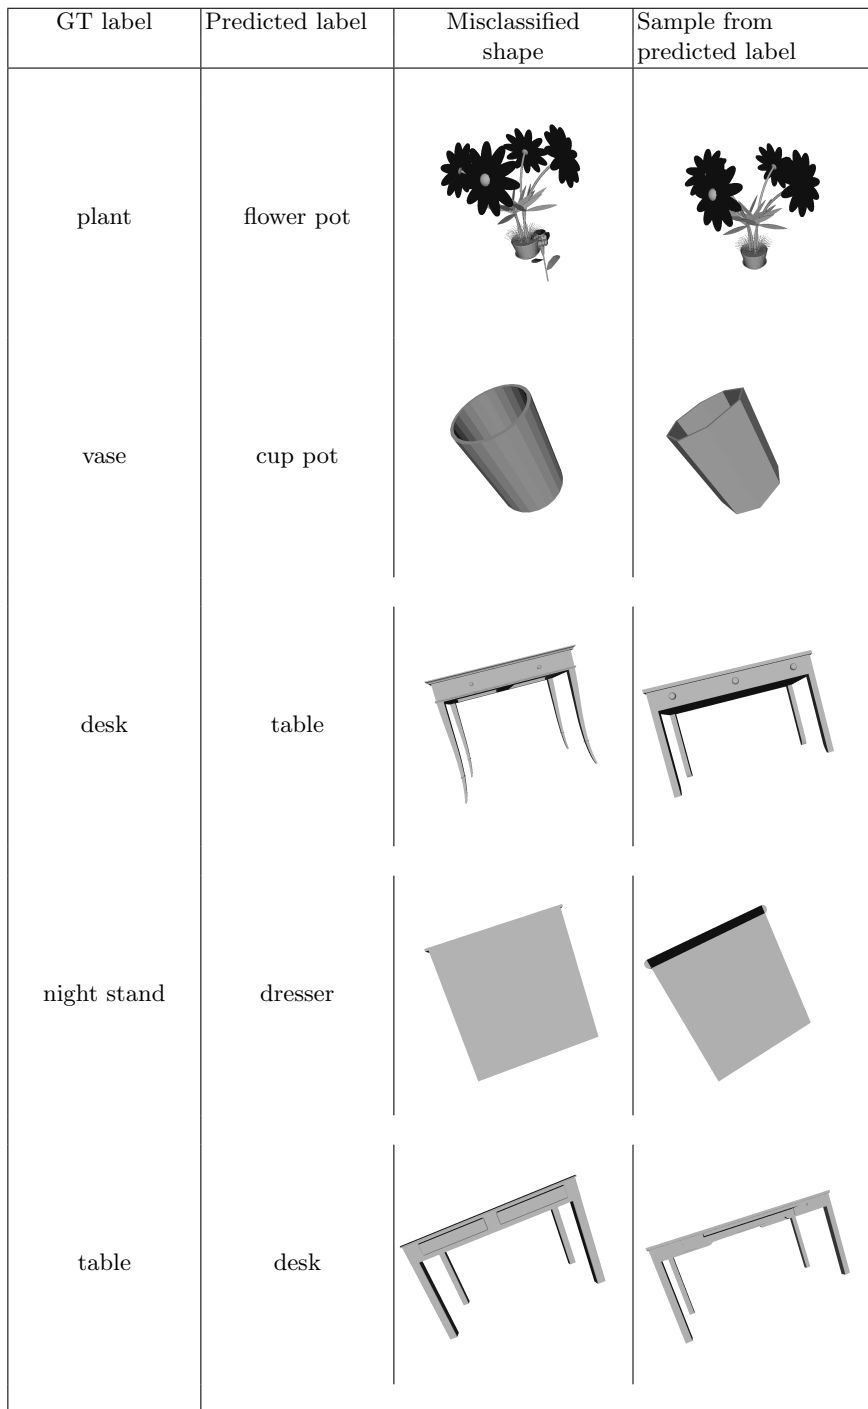  | 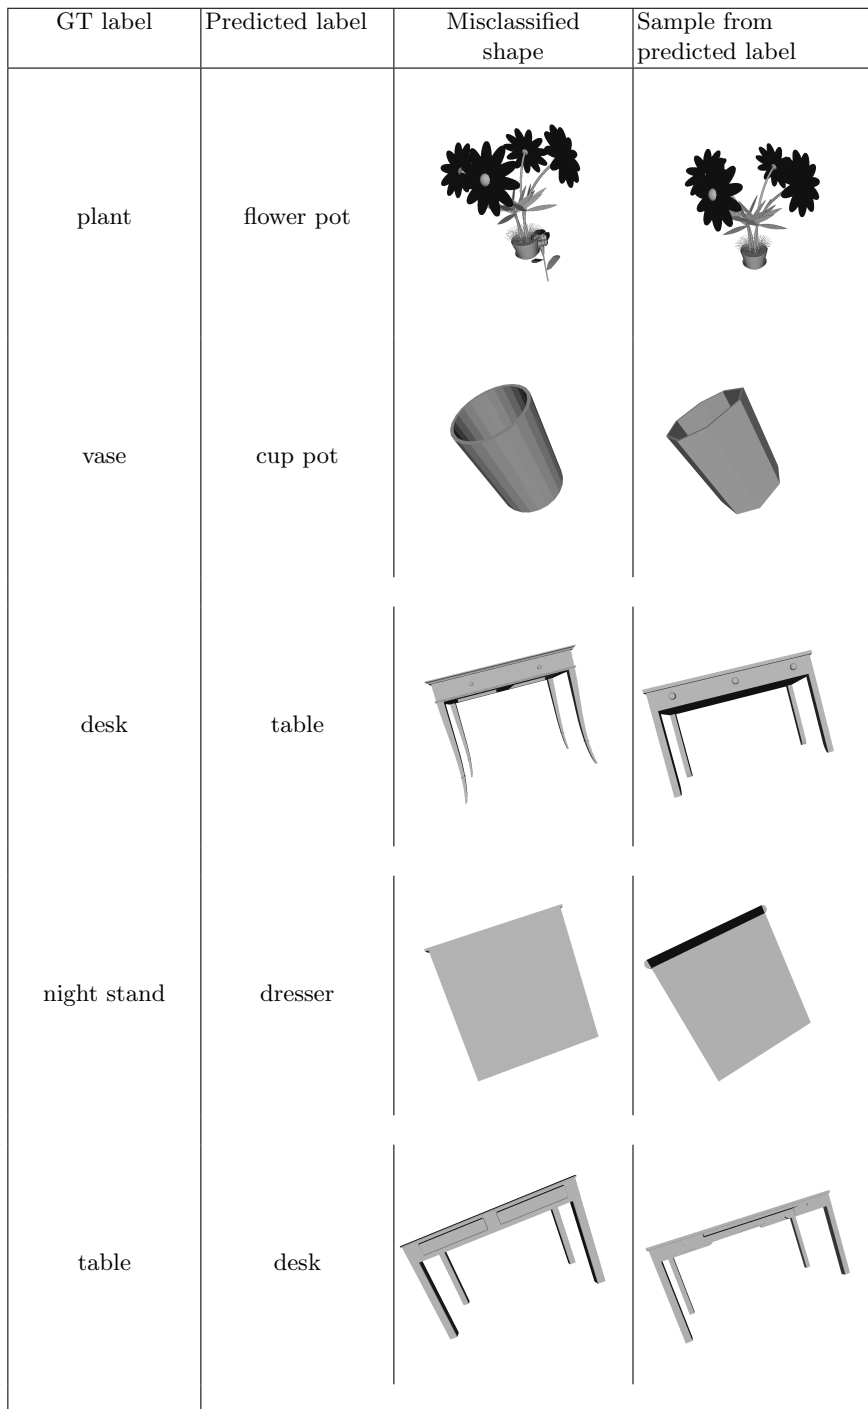  |
| table       | desk            | 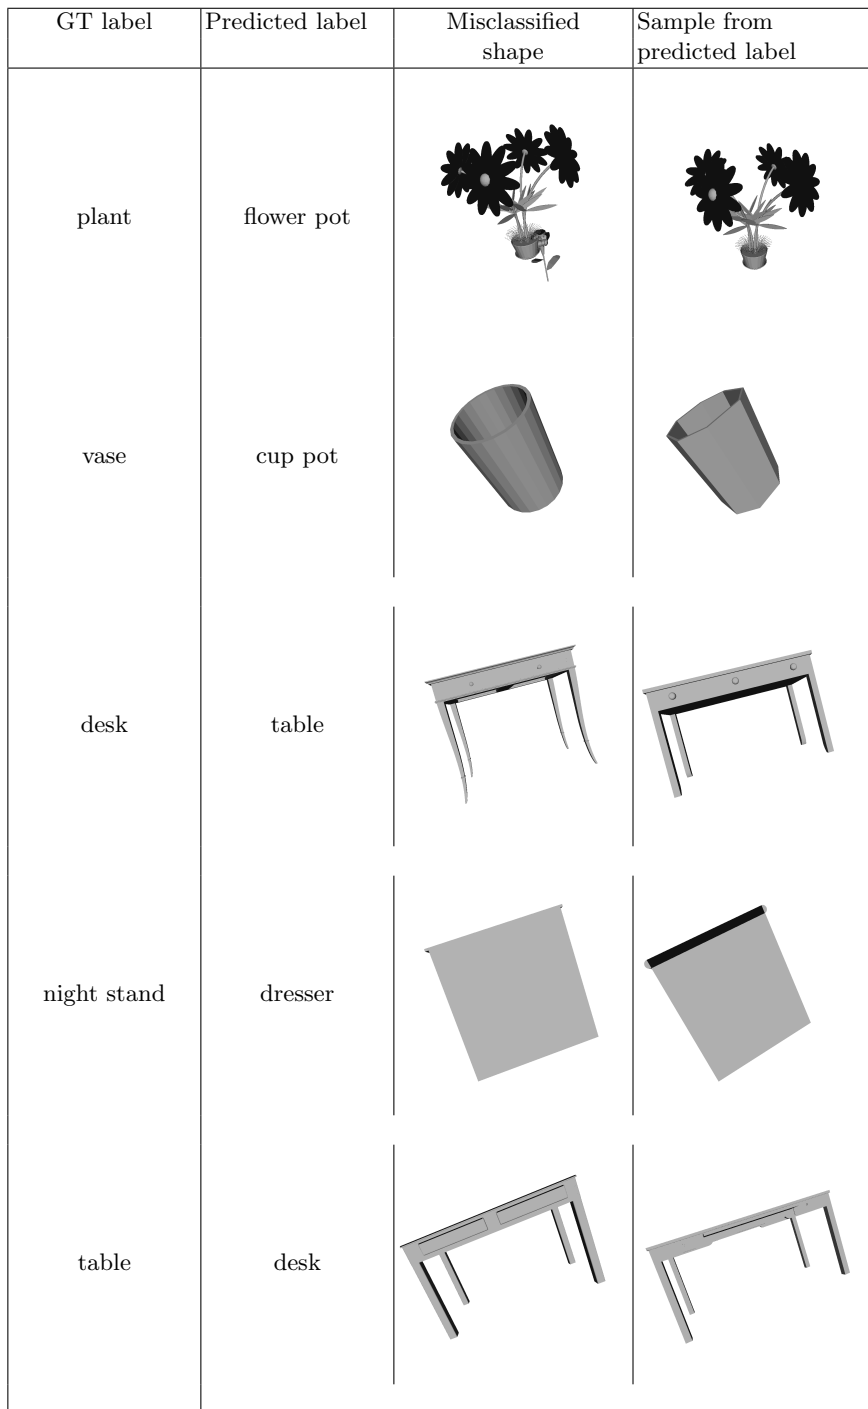 | 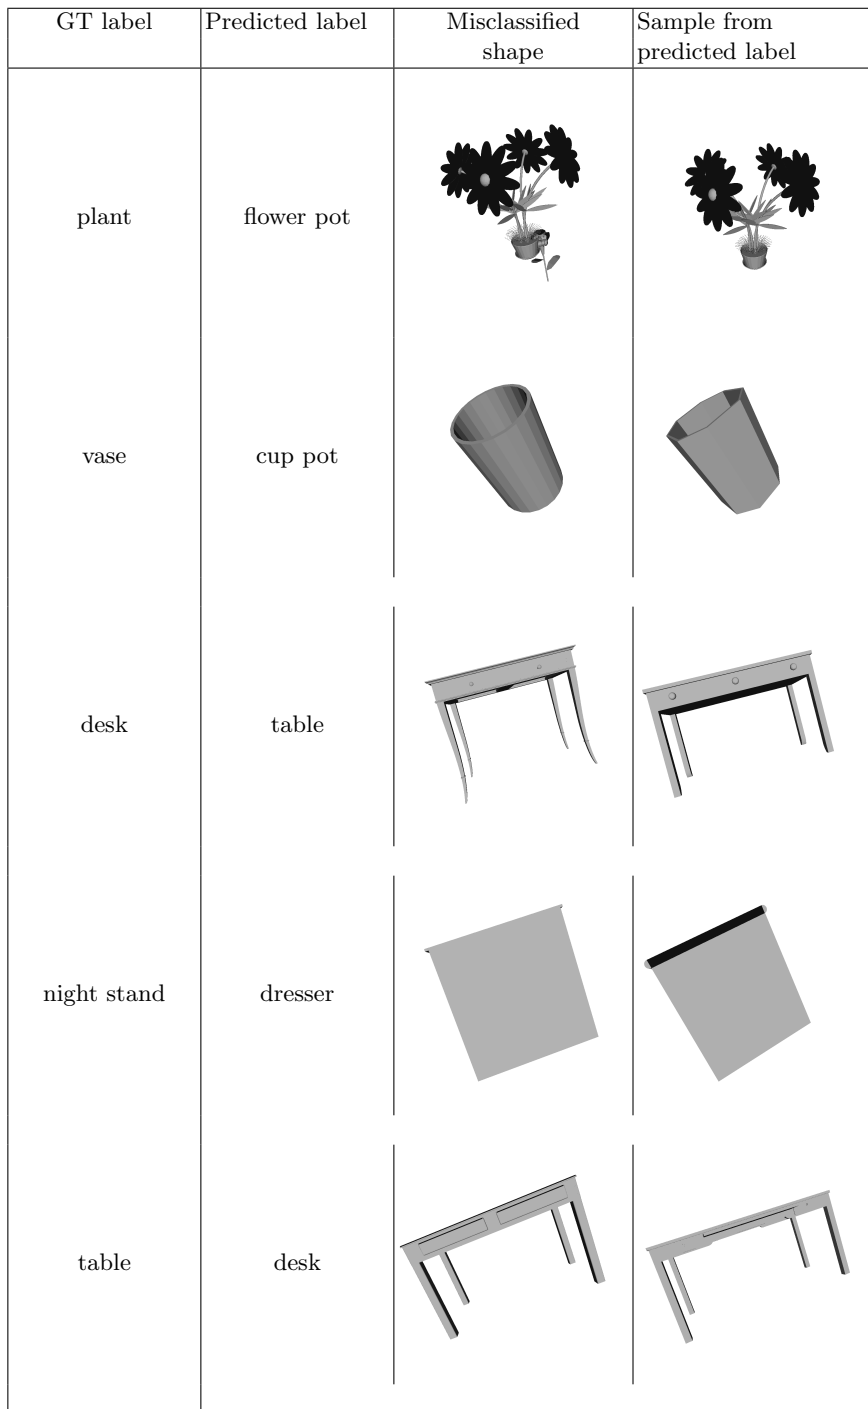 |

Table 4: Example of misclassified shapes and a close looking sample from its predicted label in ModelNet40.
